# Supplementary material for: Searching for Robustness: Loss Learning for Noisy Classification Tasks
Source: arXiv:2103.00243 source file (2021-02-27)
Supplement: Supplementary file 1 [file 7_appendix.tex]

\section{Appendix}
\subsection{Experiment dataset \label{aped: dataset}}
\begin{table}[ht]\footnotesize
\centering
\caption{The datasets used in the experiments.}
\begin{tabular}{c|c|c|c|c}
\hline
\hline
 & number of training & number of test & number of class & image size \\
\hline
\textsl{MNIST} &  60,000 & 10,000 & 10 & $28 \times 28$ \\
\hline
\textsl{KMNIST} &  60,000 & 10,000 & 10 & $28 \times 28$ \\
\hline
\textsl{CIFAR-10} &  50,000 & 10,000 & 10 & $32 \times 32$ \\
\hline
\textsl{CIFAR-100} &  50,000 & 10,000 & 100 & $32 \times 32$ \\
\hline
\textsl{Clothing1M} &  1,000,000 & 10,000 & 14 & $224 \times 224$ \\
\hline
\hline
\end{tabular}
\end{table}
\subsection{Taylor Polynomial \label{aped: taylor}}
The $4^{th}$ order taylor series:
\begin{align}
\mathcal{L}(\vec{\hat{y}}, \vec{y}) =& \vec{\theta}_2(\vec{\hat{y}}_i - \vec{\theta}_0) + \frac{1}{2}\vec{\theta}_3(\vec{\hat{y}}_i - \vec{\theta}_0)^2 +\frac{1}{6}\vec{\theta}_4(\vec{\hat{y}}_i - \vec{\theta}_0)^3 + \frac{1}{24}\vec{\theta}_5(\vec{\hat{y}}_i-\vec{\theta}_0)^{4}\nonumber\\
    & + \vec{\theta}_6(\vec{\hat{y}}_i - \vec{\theta}_0)(\vec{y}_i - \vec{\theta}_1) + \frac{1}{2}\vec{\theta}_7(\vec{\hat{y}}_i-\vec{\theta}_0)(\vec{y}_i -\vec{\theta}_1)^2 + \frac{1}{2} \vec{\theta}_8(\vec{\hat{y}}_i - \vec{\theta}_0)^2(\vec{y}_i - \vec{\theta}_1)  \nonumber \\
    & + \frac{1}{6}\vec{\theta}_9(\vec{\hat{y}}_i - \vec{\theta}_0)^3(\vec{y}_i - \vec{\theta}_1)+\frac{1}{6}\vec{\theta}_{10}(\vec{\hat{y}}_i - \vec{\theta}_0)(\vec{y}_i - \vec{\theta}_1)^3 + \frac{1}{4}\vec{\theta}_{11}(\vec{\hat{y}}_i - \vec{\theta}_0)^2(\vec{y}_i - \vec{\theta}_1)^2\nonumber \\
    & + \vec{\theta}_{12}(\vec{y}_i - \vec{\theta}_1) + \frac{1}{2}\vec{\theta}_{13}(\vec{y}_i - \vec{\theta}_1)^2 +\frac{1}{6}\vec{\theta}_{14}(\vec{y}_i - \vec{\theta}_1)^3 + \frac{1}{24}\vec{\theta}_{15}(\vec{y}_i-\vec{\theta}_1)^{4} \nonumber
\end{align} 
\subsection{Architecture of Neural networks \label{aped:arch}}
The network architectures of the MLP and CNN models used in the experiments part.
\begin{table}[ht]
\centering
\footnotesize
%\top
\caption{The architectures used in the experiments}
\begin{tabular}{ c|c|c|c|c}%{p{3.5cm}<{\centering}|p{3.5cm}<{\centering}}
\midrule
\midrule
2-Layer MLP & 3-Layer MLP & 4-Layer CNN & JoCoR-Net \\
\midrule
$28 \times 28$ Gray Image & $28 \times 28$ Gray Image &   $32 \times 32$ RGB Image& $32 \times 32$ RGB Image\\
\midrule
%\multirow{6}*{FC $28 \times 28 \longrightarrow 256$, ReLU } & 
\multirow{6}*{FC $28 \times 28 \longrightarrow 256$, ReLU } & 
%\multirow{6}*{FC $28 \times 28 \longrightarrow 256$, ReLU } 
\multirow{3}*{ FC $28 \times 28 \longrightarrow 256$, ReLU}
& 
\tabincell{c}{$5 \times 5$, 32, ReLU}
&
\tabincell{c}{$3 \times 3$, 64 BN, ReLU \\ $3 \times 3$, 64 BN, ReLU \\ $2 \times 2$ Max-pool} \\ 
\cline{4-4} & \multirow{3}*{FC$256\longrightarrow 256$, ReLU} & \tabincell{c}{$5 \times 5$, 64, ReLU} & \tabincell{c}{$3 \times 3$, 128 BN, ReLU \\ $3 \times 3$, 128 BN, ReLU \\ $2 \times 2$ Max-pool} \\
\cline{4-4} & & \tabincell{c}{FC $ 1024 \longrightarrow 1024$, ReLU} &\tabincell{c}{$3 \times 3$, 196 BN, ReLU \\ $3 \times 3$, 196 BN, ReLU \\ $8 \times 8$ Avg-pool} \\
\midrule
FC $ 256 \longrightarrow 10$&  FC $256\longrightarrow 10$ & FC $1024\longrightarrow 10$   & FC $ 196 \longrightarrow 100$ \\
\bottomrule
\end{tabular}
\end{table}
